# Supplementary material for: The Option Value of Contract Duration: Evidence from the U.S. Timber Market
Source: arXiv:2412.20285 source file (2025-12-10)
Supplement: Supplementary file 1 [file 07_appendix.tex]

\section{Appendix}\label{sec:appendix}
\subsection{Risk averse bidders}
We recover a risk-averse parameter of a constant relative risk aversion (CRRA) specification from both oral and sealed bid auction formats as a benchmark using \cite{lu2008estimating}. 
The risk-averse parameter $\theta$ nests a risk-averse ($\theta=0$) and risk-neutral ($\theta=1$). 
We use auctions in which two active bidders exist and parametrically estimate value distribution conditional on observed auction-level characteristics from oral auctions because the sample size of auctions in which more than three bidders exist is small, as shown in Table \ref{tb:summary_statistics_of_entry_and_bidding_stage}. 
As a result, our recovered risk-averse parameter is 0.507 which implies significant risk-averse bidding behaviors in the timber auctions.

\subsection{Compute bidding functions}
In Section \ref{sec:counterfactual}, we compute equilibrium bidding functions in the first-price sealed-bid auctions for different bidders' types. Note that we have two-type bidders: loggers and sawmills. Let $N_l$ ($N_s$) be the number of type-$l$ ($s$) bidders. Total number of bidders is defined by $N=N_l + N_s$. We consider the problem that type-s bidder $i$ solves the following maximization problem:
\begin{equation*}
    \max_{b_{i,s}} (v_i - b_{i,s}) F_s(v_s(b_{i,s}))^{N_s-1}F_l(v_l(b_{i,s}))^{N_l}.   
\end{equation*}
We obtain the following first order condition:
\begin{align}\label{eq:foc_types}
&F_s(v_s)^{N_s-1}F_l(v_l)^{N_l}  \nonumber \\ 
&\quad =   (v_i - b^*_{i,s})\left\{(N_s-1)F_s(v_i)^{N_s-2}f_s(v_s)v'_s(b^*_{i,s})F_l(v_l)^{N_l} + N_l F_l(v_i)^{N_l-1}f_l(v_l)v'_l(b^*_{i,s})F_s(v_s)^{N_s-1}\right\} \nonumber \\  
&\frac{1}{v_i - b^*_{i,s}} \nonumber \\  
&\quad = \frac{(N_s -1 )f_s(v_s)}{F_s(v_s)}v'_s(b^*_{i,s}) + \frac{N_l f_l(v_l)}{F_l(v_l)}v'_l(b^*_{i,s}).
\end{align}
We solve a similar problem for the type-$l$ bidder and obtain the following first order condition:
\begin{align}\label{eq:foc_typel}
    \frac{1}{v_i - b^*_{i,l}} = \frac{(N_l -1 )f_l(v_l)}{F_l(v_l)}v'_l(b^*_{i,l}) + \frac{N_s f_s(v_s)}{F_s(v_s)}v'_s(b^*_{i,l}).
\end{align}
By arranging (\ref{eq:foc_types}) and (\ref{eq:foc_typel}), we obtain the following system of equations:
\begin{align}\label{eq:foc_bidding}
\begin{split}
    v'_s - \frac{F_s}{f_s}\frac{1}{N - 1}\left(\frac{N_l}{v_l-b} + \frac{N_s-1}{v_s-b} \right) &=0\\
    v'_l - \frac{F_l}{f_l}\frac{1}{N - 1}\left(\frac{N_s}{v_s-b} + \frac{N_l-1}{v_l-b} \right) &=0.
\end{split}
\end{align}

The goal of this appendix is to numerically recover the bidding function for each type. The numerical methods are developed in the computational economics literature, and you can refer to \cite{hubbard2014numerical} for the comprehensive survey. Among the various methods, we follow \cite{hubbard2013using} to compute the inverse bidding function $\phi_m$. Their approach is based on the Mathematical Programming with Equilibrium Constraints (MPEC) approach and use the following constraints found on the boundary: for all type $m\in \{s,l\}$,
\begin{align}\label{eq:condition1}
\begin{split}
    \psi_m(\underline{b}) = \underline{v};\\
    \psi_m(\bar{b}) = \bar{v}
\end{split}
\end{align}

\begin{align}\label{eq:condition2}
\begin{split}
    \sum^{N}_{j\neq i}(\bar{v}-\bar{b})f_{m(j)}(\bar{v})\psi'_{m(j)} (\bar{b}) &= 1; \\
    \psi'_m (\underline{b}) = N/(N-1),
\end{split}
\end{align}
where $\bar{b}$ denotes the bid submitted by bidders with the highest value, which is unknown. The conditions in $(\ref{eq:condition1})$ is given by the assumption that the highest (lowest) bid is submitted by bidders with the highest (lowest) value. The first of (\ref{eq:condition2}) directly follows $(\ref{eq:foc_bidding})$, and the second of (\ref{eq:condition2}) follows \cite{FIBICH2002283}. We also have inequality conditions such as

\begin{align}\label{eq:condition3}
\begin{split}
    \psi_m(b)<\psi_m&(b') \text{ if } b < b'; \\
    &b \leq \psi_m (b) , 
\end{split}
\end{align}
where the first inequality indicates a monotone bidding function, and the second inequality means that rational bidders submit bids less than their value. In summary, our ultimate goal is to solve for the inverse bid function $\psi(\cdot)$ that satisfies $(\ref{eq:foc_types})$ and $(\ref{eq:foc_typel})$ subject to the system of equations $(\ref{eq:condition1})-(\ref{eq:condition3})$ and recover $\bar{s}$ simultaneously.

However, it is hard to verify whether $\psi(\cdot)$ satisfies the aforementioned conditions over every point. Therefore, \cite{hubbard2013using} introduce the approximation of $\psi(\cdot)$ using Chebyshev polynomials. The approximate inverse bid function can be expressed as

\begin{equation}
    \hat{\psi}(s; \boldsymbol{\alpha}, \bar{s}) = \sum^{K}_{k=0}\alpha_k \mathbb{T}_k[x(b;\bar{b})],
\end{equation}
where $\alpha_k$ and $\mathbb{T}_k$ represent the $k$-th Chebyshev coefficient and polynomial, and $x(s;\bar{s})$ lies in the interval between $-1$ and $1$. These are specified as follows:
\begin{align}
    \begin{split}
        \mathbb{T}_0(x)&=1 ;\\
        \mathbb{T}_1(x)&=x ;\\
        \mathbb{T}_{k+1}(x)&=2x\mathbb{T}_{k}(x)-\mathbb{T}_{k-1}(x);
        x_t
    \end{split}
\end{align}

\begin{align}
    \begin{split}
        x_t = \cos \left(\frac{2t-1}{2T}\pi \right) 
    \end{split}
\end{align}
The points ${b_t}$ are found using the following transformation:
\begin{align}
    \begin{split}
        x_t :=& x(b_t;\bar{b}) = \frac{2b-\underline{v}-\bar{b}}{\bar{b} - \underline{v}}; \\
        b_t =& \frac{\bar{b}+\underline{v}+(\bar{b}-\underline{v})x_t}{2}.
    \end{split}
\end{align}
When we solve for Chebyshev coefficients, we use the following objective function:
\begin{align}
\begin{split}
    &\omega_{\text{FOC}}\sum_{n}\sum_{t} \left[\text{left-hand side of }(\ref{eq:foc_bidding}) \text{ in each grid }t \right]  \\
    &\quad\quad + \omega_{\underline{v}}(\psi_m(\underline{b}) - \underline{v}) +  \omega_{\bar{v}}(\psi_m(\bar{b}) - \bar{v})\\
    & \text{subject to the inequality conditions } (\ref{eq:condition3}),
\end{split}
\end{align}
where each $\omega$ represents the weight of each constraint. We do not include the constraints in $(\ref{eq:condition2})$ because they are automatically satisfied if the first-order condition $(\ref{eq:foc_bidding})$ holds. In our counterfactual, we set $(\omega_{\text{FOC}},\omega_{\underline{v}},\omega_{\bar{v}})= (0.6,0.2,0.2)$ and $K=7$.  
